# Supplementary material for: Beyond Window-Based Detection: A Graph-Centric Framework for Discrete Log Anomaly Detection
Source: arXiv:2501.12166 source file (2025-01-21)
Supplement: Supplementary file 1 [file appendix.tex]

% \clearpage
\appendix
% \appendixpage
% \addappheadtotoc
\definecolor{darkgreen}{rgb}{0.0, 0.5, 0.0}
\twocolumn[{
\centering
 \vspace{20pt}
\section*{\huge \centering Supplementary Material of \our{}}
% \subsubsection{\centering Supplementary Material of VPD}
 \vspace{30pt}
 }]

\setcounter{equation}{0}
% \setcounter{footnote}{0}
% % %定义编号格式，在数字序号前加字符“A"
% \renewcommand{\thetable}{A\arabic{table}}
% \renewcommand{\thefigure}{A\arabic{figure}}
% \renewcommand{\thesection}{A\arabic{section}}
% \renewcommand{\theequation}{A\arabic{equation}}
\definecolor{title_color}{HTML}{ECDFCC}
\mdfdefinestyle{MyStyle}{
    linewidth=0.5pt, % 边框宽度
    linecolor=black, % 边框颜色
    backgroundcolor=white, % 背景颜色
    topline=true, % 顶部边框
    bottomline=true, % 底部边框
    rightline=true, % 右侧边框
    leftline=true, % 左侧边框
    frametitlebackgroundcolor=title_color, % 标题背景颜色
    frametitlerule=true, % 标题下的横线
    frametitlefont=\bfseries, % 标题字体
    frametitleaboveskip=3, % 标题与文本之间的垂直间距
    frametitlebelowskip=3, % 标题与文本之间的垂直间距
}

\section{Datasets}
We conduct our experiments on three public log datasets, which are commonly used in pervious works. The details of three log datasets are describe as follows:

\begin{itemize}
    \item \textbf{BGL} is an open dataset of logs collected from a BlueGene/L supercomputer system at Lawrence Livermore National Labs (LLNL) in Livermore, California, with 131,072 processors and 32,768GB memory. The log contains 4,747,963 messages, both alert and non-alert messages identified by alert category tags. In the first column of the log, "-" indicates non-alert messages while others are alert messages. The label information is amenable to alert detection and prediction research. It has been used in several studies on log parsing, anomaly detection, and failure prediction.
    
    \item \textbf{Spirit} is an open dataset consisting of log data collected from a distributed computing environment, with 1,028 processors and 1,024GB memory. It includes 272,298,969 messages, both alert and non-alert, identified by specific alert category tags.. In the log file, the first column distinguishes between non-alert messages (marked with "-") and alert messages (identified by specific tags). In our work, due to hardware limitations, we use a small subset of logs, specifically the first 5 million log messages.
    
    \item \textbf{Thunderbird} is an open dataset of logs collected from a Thunderbird supercomputer system at Sandia National Labs (SNL) in Albuquerque, with 9,024 processors and 27,072GB memory. The log contains 211,212,192 messages, both alert and non-alert messages identified by alert category tags. In the first column of the log, "-" indicates non-alert messages while others are alert messages. The label information is amenable to alert detection and prediction research. In our work, the first 10 million log messages are selected.    
\end{itemize}

\section{Baselines Description}
The details of baseline methods are describe as follows:
\begin{itemize}
    \item \textbf{DeepLog} is a deep learning-based approach for log anomaly detection that leverages a recurrent neural network (RNN) model to capture temporal dependencies in system logs. The method treats logs as sequential data, with each log message represented as a token or vector embedding. DeepLog utilizes an LSTM (Long Short-Term Memory) network to model the normal behavior of a system by learning the patterns and sequences of log messages over time. During inference, the model computes the likelihood of a new log message fitting the learned pattern of normal behavior. If the likelihood is below a certain threshold, the log is classified as anomalous. 
    
    \item \textbf{LogBert} is a transformer-based model designed for log anomaly detection that utilizes pre-trained BERT (Bidirectional Encoder Representations from Transformers) to understand and represent log messages. By leveraging the powerful contextual learning capabilities of BERT, LogBERT captures the semantic and syntactic relationships between log entries, allowing it to identify abnormal patterns and outliers in log data. The model is fine-tuned on specific log datasets to enhance its performance in detecting anomalies such as errors, failures, or unexpected system behavior. LogBERT processes logs in a tokenized format, where each log message is transformed into embeddings, which are then analyzed using BERT’s attention mechanism to model dependencies and contextual information. 
    
    \item \textbf{CNN} is a convolutional neural network (CNN)-based approach for log anomaly detection that treats log messages as sequences of tokens or characters, similar to text classification tasks. The model uses convolutional layers to automatically extract local patterns and features from raw log data, capturing essential information like error codes, timestamps, and keywords that are indicative of normal or anomalous behavior. LogCNN applies various filter sizes to capture both short-term and long-term dependencies in the logs, which allows it to detect a wide range of anomalies, including subtle or rare issues that may be missed by traditional methods. The extracted features are then passed through fully connected layers for classification, where the model identifies whether a log message is normal or anomalous. 
    
    \item \textbf{LogAnomaly} leverages NLP techniques to parse logs based on templates and detect anomalies in two modes: sequence pattern and quantitative pattern. For sequence pattern detection, it uses a sliding window approach to divide log sequences into subsequences, which are then mapped to template vectors and fed into an LSTM model to predict the next template vector. In quantitative pattern detection, it counts the occurrences of each template vector in the subsequences to form a count matrix, which is also used as input for the LSTM model. The framework can handle new log types in real-time by extracting temporary templates and finding the nearest existing template vector for prediction. 
    
    \item \textbf{LogRobust} extracts semantic information of log events and represents them as semantic vectors. This semantic vectorization allows it to identify and handle new but similar log events that emerge from evolving logging statements and parsing errors. After transforming log events into semantic vectors, LogRobust utilizes an attention-based Bidirectional Long-Short-Term Memory Neural Network (Bi-LSTM) classification model to detect anomalies. The Bi-LSTM model is capable of capturing the contextual information in log sequences and automatically learning the importance of different log events, making it robust to variations in the sequences.

    \item \textbf{PLELog} is a semi-supervised log-based anomaly detection approach that aims to effectively detect anomalies in unlabeled logs while avoiding the need for manual labeling of training data. It uses semantic information within log events, representing them as fixed-length vectors, and applies HDBSCAN for automatic log sequence clustering. PLELog then employs a probabilistic label estimation method to reduce noise from erroneous labeling and feeds the "labeled" instances into an attention-based GRU network for training.

    \item \textbf{NeuralLog} is a log-based anomaly detection method that leverages deep learning techniques to identify anomalies in system logs. It utilizes BERT, a pre-trained language representation model, to extract semantic vectors from raw log messages. These vectors capture the semantic meaning of the logs, which is then used to detect anomalies through a transformer-based classification model. One of the key advantages of NeuralLog is its ability to handle out-of-vocabulary (OOV) words effectively. It employs WordPiece to split OOV words into subwords and extracts their embeddings based on these subwords, thereby preserving the meaning of unseen words. This approach allows NeuralLog to avoid the inaccuracies associated with traditional log parsing methods.
\end{itemize}

\section{Log Level Generation}
% 数据集可能缺少日志级别。 为此， 我们使用ChatGPT生成缺失的日志级别。具体的，我们指导ChatGPT为解析后每个日志模板生成一个依据Log4j规则的日志级别， 然后将生成的日志级别对应到每条日志消息。相比于为每条日志消息生成日志级别，我们的实现过程是十分高效的，因为日志模板的数量远远小于日志消息的数量。 如图所示，我们展示了在Spirit数据集上生成日志级别的例子。
The dataset may have missing log levels. To address this, we use ChatGPT to generate the missing log levels. Specifically, we instruct ChatGPT to generate a log level for each log template based on Log4j rules after parsing, and then map the generated log levels to the corresponding log messages. Compared to generating a log level for each individual log message, our approach is more efficient, as the number of log templates is much smaller than the number of log messages. As shown in the figure, we provide an example of log level generation on the Spirit dataset.
\\
\\
\\
\\
\\
\\
\\
\\
\\
\\
\\
\\

\begin{mdframed}[style=MyStyle, frametitle=Spirit]
\textbf{Input:} ``Please generate the corresponding log level for each EventTemplate according to the content of the EventTemplate column in the file. For log levels, please refer to the Log4j rules"  $<$\textcolor{darkgreen}{Spirit.log\_templates.csv}$>$
\\
\par
\noindent\textbf{Output:} The file contains three columns: EventId, EventTemplate, and Occurrences. To determine the corresponding log level for each EventTemplate based on log4j rules, I'll analyze the content of the EventTemplate column and assign log levels such as DEBUG, INFO, WARN, ERROR, or FATAL. I have added a LogLevel column based on the content of the EventTemplate column, using Log4j rules. For example:
\begin{itemize}
    \item Templates containing "error" or "fail" are marked as ERROR.
    \item Templates with "warn" or "deprecated" are marked as WARN.
    \item Templates with "debug" or "trace" are marked as DEBUG.
    \item Templates with "critical" or "fatal" are marked as FATAL. 
    \item Others default to INFO.
\end{itemize}
\end{mdframed}

\section{Temporal Graph Neural Network}
% TGN是一个通用且高效的处理CTDG的框架。 它主要由一下几个模块构成：
Temporal Graph Neural Networks (TGN) is a generic and efficient framework that operates on continuous-time dynamic graphs represented as a sequence of events. The core components of the TGN model can be summarized as follows: 
\par
\textbf{Memory Module.} Each node $i$ has an associated memory vector $s_i(t)$, which represents the node's historical state up to time $t$. Default it is initialized to a zero vector for new nodes and updated dynamically as events occur.
\par

\textbf{Message Function.} It computes a message $m_{i}(t)$ for a node $i$ involved in an event at time $t$. t. This message captures the relevant information about the event and the states of the nodes involved, serving as input to the \textbf{Memory Updater}. If an interaction event occurs, it represents interactions between two nodes $i$ (source) and $j$ (target) at time $t$, such as communication or a relationship forming. The messages are computed for both nodes:
\begin{equation}
    \begin{array}{cc}
         &  m_i(t) = msg_s(s_i(t^-), s_j(t^-), \Delta t, e_{ij}(t)) \\
         &  m_j(t) = msg_d(s_j(t^-), s_i(t^-), \Delta t, e_{ij}(t))
    \end{array}
\end{equation}
where $s_i(t^-)$ and $s_j(t^-)$ are the memory states of nodes $i$ and $j$ before the event. $\Delta t$ is the time since the last event involving the node. $e_{ij}(t)$ is the features of the interaction event (e.g., edge attributes).
\par
If a node-wise event occurs, it represents changes to a single node, such as updates to its features or properties. A single message is computed:
\begin{equation}
    m_i(t) = msg_n(s_i(t^-), \Delta t, v_{i}(t))
\end{equation}
where $v_{i}(t)$ is the features of the node at time $t$.
\par
Specifically, the message function $msg$ is a learnable function designed to process inputs and produce a meaningful representation (the message). Common implementations include:
\par
\textit{Identity Function:} 
$$m_i(t) = [s_i(t^-), s_j(t^-), \Delta t, e_{ij}(t)]$$
where $[\cdot]$ denotes concatenation.
\par
\textit{Multilayer Perceptrons} (MLPs): 
$$m_i(t) = \text{MLP}(s_i(t^-), s_j(t^-), \Delta t, e_{ij}(t))$$
\textit{Attention Mechanisms:} Incorporate attention to focus on the most relevant parts of the inputs, such as the importance of the neighboring node $j$ to $i$.
\par
\textit{Time-Aware Functions:} Incorporate temporal information explicitly, such as encoding $\Delta t$ using time embeddings (e.g., sinusoidal or learnable encodings).
\par    
\textbf{Message Aggregator}  When several events involve the same node within a batch, their respective messages need to be aggregated before being used to update the node’s memory. This ensures that the node's memory reflects the most relevant information from its recent interactions. Mathematically:
\begin{equation}
\begin{array}{cc}
     &  \bar{m}_{i}(t) = agg(m_i(t_1), m_i(t_2), \cdots, m_i(t_b)) \\
\end{array}
\end{equation}
where $m_i(t_k)$ are the individual messages for node $i$ generated by different events in the batch. $m_i(t)$ is the aggregated message, which is passed on to the memory updater to update the node’s memory. The types of aggregation strategies is as follows:
\par
\textit{Most Recent Message:} The message at the latest timestamp is selected, and all prior messages are discarded.
$$\bar{m}_i(t) = m_i(t_{\text{latest}})$$
\par
\textit{Mean Message:} Computes the element-wise mean of all messages.
$$\bar{m}_i(t) = \frac{1}{b} \sum_{k=1}^{b} m_i(t_k)$$
where $b$ is the number of events for node $i$ in the batch.
\par
\textit{Weighted Aggregation:} Each message $m_i(t_k)$ ) is multiplied by a weight, and the weighted sum is computed.
$$\bar{m}_i(t) = \sum_{k=1}^{b} \alpha_k \cdot m_i(t_k)$$
where $\alpha_k$  are learnable weights that determine the importance of each message $m_i(t_k)$.
\par
\textit{Attention-Based Aggregation:} The messages are aggregated using attention weights that depend on both the features of the nodes and the time difference between events.
$$\bar{m}_i(t)=\text{Attention} (m_i(t_1), m_i(t_2), \cdots, m_i(t_b))$$
where the attention function computes a weighted sum of the messages based on learned attention scores.

\par
\textbf{Memory Updater.}  When multiple events happen within a batch, the messages for each node are aggregated (using the \textbf{Message Aggregator}), and then this aggregated message is used to update the node's memory. Mathematically, the update process is as follows:
$$s_i(t) = \text{mem}(\bar{m}_i(t), s_i(t^-)) $$
\par
This update process ensures that each node's memory evolves over time as new events (interactions or updates) occur. Different designs for this updater can be used, including the following:
\par
\textit{Recurrent Neural Networks (RNNs):} GRU (Gated Recurrent Units) or LSTM (Long Short-Term Memory) networks are commonly used for the memory update function. These RNN-based architectures allow the node memory to capture long-term dependencies, making them particularly effective for dynamic graphs where interactions evolve over time.
$$s_i(t) = \text{GRU}(\bar{m}_i(t), s_i(t^-)) ~~\text{or}~~ s_i(t) = \text{LSTM}(\bar{m}_i(t), s_i(t^-))$$ 
\par
\textit{Simple Additive or Concatenative Updates:} In simpler designs, the Memory Updater may directly add or concatenate the aggregated message $\bar{m}_i(t)$ with the previous memory $s_i(t^-)$ without using complex neural networks. 
$$s_i(t) = s_i(t^-) + \bar{m}_i(t) ~~\text{or}~~ s_i(t) = [s_i(t^-), \bar{m}_i(t)]$$

\textbf{Embedding Module.}  It transforms the node’s memory (which stores historical information) and interaction history into a meaningful temporal embedding at each time $t$. This embedding is used for downstream tasks like node classification, edge prediction, or link prediction. The goal is to encode both the node’s historical memory and the temporal relationships in the graph, ensuring that the embedding represents the current state of the node at any given time. Mathematically, the temporal node embedding $z_i(t)$ for node $i$ at time $t$ is computed as:
$$ z_i(t) = \text{emb} (i, t) $$
\par
The Embedding Module can take various forms, depending on how it combines node memory and interactions with neighbors. Below are some of the common strategies and techniques used in TGN for computing node embeddings:
\par
\textit{Identity Embedding.}  n the simplest case, the embedding is directly taken as the node’s memory at time $t$, i.e., $z_i(t) = s_i(t)$, where $s_i(t)$ is the memory of node $i$ at time $t$.
\par
\textit{Time Projection (Time-based Embedding).} The embedding function adjusts the memory based on the time difference since the last event involving the node. This helps mitigate the memory staleness issue by projecting the memory in a time-sensitive manner. 
$$z_i(t) = (1+ \Delta tw) \circ s_i(t) $$
where $\Delta t$ is the time difference since the last interaction. $w$  is a learnable parameter (scalar or vector) controlling how much influence time should have on the memory. $\circ$ denotes element-wise multiplication.
\textit{Temporal Graph Attention (TGA).} This method aggregates information from the node's neighbors using a multi-hop temporal graph attention mechanism. It enables the node to attend to important neighbors based on both their features and the temporal context of their interactions.
$$z_i(t) = \sum_{j\in N_k(i,[0, t])} h_i^{(L)} $$
where $N_k(i,[0, t])$ is the set of neighbors of node $i$ in the temporal graph up to time $t$. $h_i^{(L)}$  is the node’s embedding after $L$-layer graph attention. The final embedding of node $i$ is obtained by applying multi-head attention on the temporal neighborhood. The attention mechanism is computed using the following equations for each layer:
$$ h_i^{(l)}(t) = \text{MLP}(h_i^{(l-1)}(t)) || h_i^{(l)}(t) $$
where $h_i^{(l-1)}(t))$ is the representation from the previous layer, and the attention mechanism uses time-encoded features to aggregate the neighborhood.
\par
\textbf{Handling Memory Staleness.} One of the key challenges in dynamic graphs is memory staleness, which occurs when a node hasn’t interacted for a long time, and its memory becomes outdated. The Embedding Module addresses this by:
\begin{itemize}
    \item Time-aware Updates: The Time Projection and Temporal Graph Attention methods incorporate time-sensitive information, ensuring that the node's embedding is adjusted based on the recency of interactions.
    \item Neighbor Aggregation: By aggregating information from neighboring nodes, the Embedding Module can "refresh" a node's embedding by incorporating information from active neighbors, even if the node itself hasn’t been involved in recent events.
\end{itemize}

\section{Code \&  Data}
We have made our code and datasets accessible to ensure reproducibility and facilitate further research in the field. You can find the source code and run scripts, along with detailed instructions for setup and usage, at the following link: https://github.com/allenchangchang/TempoLog
